# Supplementary material for: Automated Verification of CountDownLatch
Source: arXiv:1908.09758 source file (2019-08-26)
Supplement: Supplementary file 1 [file appendix.tex]

\hide{
\section{Programming Language}
\label{sec:proglang-app}

We use the core programming language in Fig.~\ref{fig.proglang}
to convey our idea.
A program consists of
data declarations ($\nonterm{data\_decl}^*$),
global variable declarations ($\nonterm{global\_decl}^*$),
and procedure declarations ($\nonterm{proc\_decl}^*$).
Each procedure declaration is annotated with
pairs of pre/post-conditions ($\constr_{pr}/\constr_{pr}$).
New objects of type \term{C} can be dynamically created and destroyed
using  \lit{new} and \lit{destroy}.
A \lit{fork} receives a procedure name \nonterm{pn} and
a list of parameters $\term{v}^*$, creates a new thread
executing the procedure \nonterm{pn}, and returns
an object of {\bf thrd} type representing the newly-created
thread.
$\lit{join} \lit{(} \term{v} \lit{)}$ waits for the thread
pointed to by \term{v} to finish its execution.
Note that a joinee could be joined in multiple joiners.
At run-time, the joiners wait for the joinee to complete
its execution. If a joiner waits for an already-completed thread,
it proceeds immediately without waiting (i.e. the join
operation becomes no-op).
%% Following mainstream languages such as Java, C\#, and C/C++,
We do not allow canceling a thread abruptly.
A thread is destroyed
when it is joined or when the entire program has finished
its execution.
The semantics of other program statements (such as procedure
calls $\nonterm{pn} \lit{(} \term{v}^* \lit{)}$,
conditionals, loops, assignments) are standard as can be found in
the mainstream languages. The operational semantics of programs
written in our language
is defined in Appendix~\ref{sec:semantics}.

\section{Operational Semantics}
\label{sec:semantics}

In this section, we define the interleaving operational semantics of programs
with fork/join concurrency. Our semantics resembles the semantics
of well-known concurrent languages such as Java, C\#, and C/C++.

\begin{mydef}[Well-formness]
A program is well-formed if the following conditions hold:
\begin{itemize}
  \item In the program text, there exists a procedure called main,
which indicates the entry point of the program.
  \item Procedure names are unique within a program. Procedure
parameters are unique within a procedure. Free variables
in the body of a procedure are the procedure parameters.
  \item A normal procedure call or a fork statement mentions
only procedure names defined in the program text.
The number of actual parameters and formal parameters
are equal.
\end{itemize}
\end{mydef}

A thread can be in one of three states: \myit{running}, \myit{dead}, and \myit{aborted}.
Our verification framework ensures that 
no thread ends up in an \myit{aborted} state.
A program state is \myit{non-aborting} if neither of threads is in an
\myit{aborted} state. A program state is \myit{final} if 
all threads are in a \myit{dead} state.

%% \savespace
\begin{mydef}[Thread State]\label{def:state}
A thread state $\state$ is one of the following states:
\begin{itemize}\savesmallspace
  \item $\lit{run}(s,\envir)$ stating that the thread is running with
remaining statement $s$ and environment $\envir$.
For brevity, $\envir$ is assumed to be 
a partial function from object names to object references and
from stack variables to values. Environment $\envir$ resembles stack
and heap in programs. An update at $v$ with $o$ in $\envir$
is denoted as $\envir [ v \mapsto o]$.
  \item $\lit{dead}$ stating that a thread has completed its execution.
  \item $\lit{aborted}$ stating a thread has performed an illegal operation,
such as null-pointer dereference.
\end{itemize}
\end{mydef}\savesmallspace

%% \savespace
\begin{mydef}[Program State]
A program state $\config$ consists of a set of threads $\threads$ where
each thread is a pair of
($\tid,\state$) representing thread identifier $\tid$ and
thread state $\state$. The thread identifier $\tid$ is of type
\code{thrd} while the thread state $\state$ is defined above.
\end{mydef}

%% \savespace
\begin{mydef}[Execution]
Execution of a program starts in the initial program state:
$(\{(\_ , \lit{run}({s},\emptyset))\})$, where
$s$ is the code fragment of the main procedure.
\end{mydef}\savesmallspace

Fig.~\ref{fig.smallstep} shows the small-step operational semantics.
A premise marked with \highlightd{\text{box}} denotes the fact that threads must
block and wait for the premise to become true. For example,
joining with a thread blocks until the thread is dead.
In Fig.~\ref{fig.smallstep},
$spec(pn)$ denotes the specification of the procedure $pn$
in the program,
$eval(e,\envir)$ denotes the evaluation of the expression $e$
in the environment $\envir$.
The rules for fork and join are of special interest.
In the fork rule, a new thread is spawned and the return
value $v$ points to its identifier $\tid_1$ of type \code{thrd}.
We explicitly add a {\myhalt} statement
%% that is automatically added
to signify the end of each newly spawned thread.
As a quick observation, a thread identifier corresponds
to a thread node in our logic.
Any threads (joiners) knowing the identifier can perform a join operation
to join with the newly-created thread (joinee).
In the join rule, if the joinee has not yet finished its execution
(i.e. it is not in a \lit{dead} state), the joiners have to wait
for the joinee to finish its execution.
Note that when a joinee is joined,
it will not be removed from the set of threads.
This allows for the multi-join pattern
and enables the
joiners to immediately proceed without waiting
in case the joinee already finished its execution.
There is a direct relation between the \lit{dead} state
of a thread during run-time and its
{\em dead} predicate during verification-time.

%%%%%%%%%%%%%%%%%%%%%%%%%%%%%%%%%%%%%%%%
\begin{figure}[!htb]
\savespace
\begin{center}
%\begin{minipage}{26pc}%{42pc}
\begin{frameit}
%% \savespace
%% \savespace
\savespace
\begin{small}
\[
\hspace{-3mm}
\begin{array}{c}
%%%%%%%%%%%%%%%%%%%%
%IF TRUE
%%%%%%%%%%%%%%%%%%%%

\begin{array}{c}

( \threadspec, \{ (\tid , \lit{run}(\lit{if} ~\nonterm{true} ~\lit{then} ~ \nonterm{$s_1$} ~ \lit{else} ~ \nonterm{$s_2$} ; s,\envir)) \} \bagunion \threads)
\to\\
( \threadspec, \{ (\tid ,\lit{run}(\nonterm{$s_1$} ; s , \envir)) \} \bagunion \threads)

\end{array} \savesmallspace \\ \\

%%%%%%%%%%%%%%%%%%%%
%IF false
%%%%%%%%%%%%%%%%%%%%

\begin{array}{c}

( \threadspec, \{ (\tid , \lit{run}(\lit{if} ~\nonterm{false} ~\lit{then} ~ \nonterm{$s_1$} ~ \lit{else} ~ \nonterm{$s_2$} ; s,\envir)) \} \bagunion \threads)
\to \\
( \threadspec, \{ (\tid ,\lit{run}(\nonterm{$s_2$} ; s , \envir)) \} \bagunion \threads)

\end{array}\savesmallspace  \\ \\

%%%%%%%%%%%%%%%%%%%%
% Ifthen else
%%%%%%%%%%%%%%%%%%%%

\begin{array}{c}
\frac{
\begin{array}{c}

eval(e,\envir)=b

\end{array}
}{
\begin{array}{c}

(\threadspec, \{ (\tid , \lit{run}(\lit{if} ~\nonterm{e} ~\lit{then} ~ \nonterm{$s_1$} ~ \lit{else} ~ \nonterm{$s_2$} ; s,\envir) ) \} \bagunion \threads)
\to \\
(\threadspec, \{ (\tid ,\lit{run}(\lit{if} ~\nonterm{b} ~\lit{then} ~ \nonterm{$s_1$} ~ \lit{else} ~ \nonterm{$s_2$} ; s , \envir)) \} \bagunion \threads)

\end{array}
}
\end{array}\savesmallspace  \\ \\

%%%%%%%%%%%%%%%%%%%%
%CALL
%%%%%%%%%%%%%%%%%%%%

\begin{array}{c}
\frac{
\begin{array}{c}

\hide{
\forall i \in \{1,\ldots,n\} \bullet \envirof{v_i} = o_i \\
}
spec(pn) := \code{pn}(w_1, \dots, w_n) ~ \lit{requires} ~\constr_{pr} ~\lit{ensures}~
\constr_{po}\lit{;} ~\{~s_{1}~\}
\\

s_1' = [v_1/w_1,\ldots,v_n/w_n]s_1

\end{array}
}{
\begin{array}{c}

( \threadspec, \{ ( \tid , \lit{run}(pn(v_1, \ldots, v_n\lit{)}; s, \envir)) \} \bagunion \threads)
\to \\
( \threadspec, \{ ( \tid , \lit{run}(s_1'; s, \envir)) \} \bagunion \threads)

\end{array}
}
\end{array} \savesmallspace \\ \\

%%%%%%%%%%%%%%%%%%%%
%FORK
%%%%%%%%%%%%%%%%%%%%

\begin{array}{c}
\frac{
\begin{array}{c}

spec(pn) := \code{pn}(w_1, \dots, w_n) ~ \lit{requires} ~\constr_{pr} ~\lit{ensures}~
\constr_{po}\lit{;} ~\{~s_{1}~\}
\\

\forall i \in \{1,\ldots,n\} \bullet \envirof{v_i} = o_i

\quad\quad

\fresh(\tid_1)

\quad\quad

\envir'= \envir [ v \mapsto \tid_1]

\\

\envir_1= [w_1 \mapsto o_1,\ldots,w_n \mapsto o_n]

\quad\quad

typeof(\tid_1)=\code{thrd}

\\

\threadspec_1 = \threadspec[ \tid_1 \mapsto \constr_{po}]

\end{array}
}{
\begin{array}{c}

( \threadspec, \{ ( \tid , \lit{run}(\nonterm{v} = \lit{fork} \lit{(} pn \lit{,} v_1, \ldots, v_n\lit{)}; s, \envir)) \} \bagunion \threads)
\to \\
( \threadspec_1, \{ ( \tid , \lit{run}(s, \envir')) \} \bagunion \{ ( \tid_1 , \lit{run}(s_1;\myhalt, \envir_1)) \} \bagunion \threads)

\end{array}
}
\end{array} \savesmallspace \\ \\
%%%%%%%%%%%%%%%%%%%%
% HALT
%%%%%%%%%%%%%%%%%%%%

\begin{array}{c}

(\threadspec, \{ ( \tid , \lit{run}(\myhalt, \envir)) \} \bagunion \threads)
\to
(\threadspec, \{ ( \tid , \lit{dead}) \} \bagunion \threads)

\end{array} \savesmallspace \\  \\

%%%%%%%%%%%%%%%%%%%%
%JOIN
%%%%%%%%%%%%%%%%%%%%

\begin{array}{c}
\frac{
\begin{array}{c}

\highlightd{ \exists ( \tid_1,\lit{dead}) \in \threads \bullet \envirof{v} = \tid_1  }

\end{array}
}{
\begin{array}{c}

( \threadspec, \{ ( \tid , \lit{run}(\lit{join} \lit{(} v \lit{)}; s, \envir)) \} \bagunion \threads)
\to
( \threadspec, \{ ( \tid , \lit{run}( s, \envir)) \} \bagunion \threads)

\end{array}
}
\end{array}  \\

\end{array}
\]
\end{small}
%% \savespace
\end{frameit}
\savesmallspace
\caption{Selected Small-step Operational Semantics of Well-formed Programs}
\label{fig:smallstep}
\savespace\savespace
%\savespace\savespace
%\end{minipage}
\end{center}
\end{figure}

%%%%%%%%%%%%%%%%%%%%%%%%%%%%%%%%%%%%%%%%

}

\hide{

\section{Improving Delayed Lockset Checking}
\label{sec:delayed-app}

In this section, we show how our ``threads as resource''
proposal could support and improve delayed
lockset checking technique proposed in \cite{Le:ATVA13}.
More specifically, the proposal makes the proof
more concise and natural, while it enables verifying
deadlock freedom of challenging programs
with non-lexical fork/join, locks, and multi-join.

\begin{figure}[!htb]
%% \savespace
%% \savespace
%% \savespace
%% \savespace
\begin{center}
\begin{minipage}{22pc}
\begin{frameit}
\savespace
%% \savespace
%% \savespace
\[
\begin{array}{rlll}

\morespace

\nonterm{type} & ::= & \ldots \mid \code{lock} & \textsf{Type}\\

\nonterm{stmt} & ::= &
	\begin{array}{ll}
	
	& \hspace{-2.3mm} \nonterm{v} = \lit{new} ~ \code{lock} \lit{(} \lit{)} \\

	\mid &  \lit{acquire} \lit{(} \nonterm{v} \lit{)} \mid 
        \lit{release} \lit{(} \nonterm{v} \lit{)}~~~~~ \\

        \mid & \ldots \\ 
			
	\end{array} & \textsf{Statement}		

\end{array}
\]
%% \savespace
%% \savespace
\end{frameit}
%\savespace
\savespace
\caption{Added Language Components for Manipulating Locks}
\label{fig.proglang-locks}
\end{minipage}
\savespace\savespace
\savespace\savespace
\savesmallspace
\end{center}
\end{figure}

Our core programming language is added with components for
manipulating non-recursive (mutex) locks\footnote{
Also called non-reentrant locks which cannot be acquired more than once.
}
(Fig.~\ref{fig.proglang-locks}).
Locks can be dynamically created and destroyed using
\lit{new} and \lit{destroy}. Locks are acquired and released
using \lit{acquire} and \lit{release}.

\input{exp-locks}

There are programs where threads' fork/join and locks' acquire/release can
interact with each other in complicated manners.
Hence, these programs are challenging to be verified as deadlock-free.
An example is the program in Fig.~\ref{fig:outline-locks}.
The key idea of the delayed lockset checking technique \cite{Le:ATVA13}
is that lockset constraints are delayed at the fork points
and they are checked at the join points instead.

%%%%%%%%%%%%%%%%%%%%%%%%%%%%%%%%%%%%%%%%
\begin{figure}[!hb]
%\savespace
\savespace
\savespace
%\savespace
\begin{center}
\begin{minipage}{25pc}%{32pc}
\begin{frameit}
\savespace
\savespace
\savespace
\[
\begin{array}{rcll}
%% \textsf{Shape predicate} & \nonterm{spred} &::=&
%% [\self{::}]\predfo{\term{c}}{\term{v}^*}{\fracperm} \veq
%% \constr~[\lit{inv}~\pure_0]\\

\textsf{Separation formula} & \constr &::=& \bigvee ( \exists v^* \cdot
\heap \wedge \pure \wedge \lockf ) \\

\textsf{Lock formula} & \lockf &::=& {\bigwedge} \locksetf \\

\textsf{Atomic heap formula} & \aheap &::=&
\permsto{\term{v}}{C({\term{v}}^*)}{\fracperm}
\mid \permsto{\term{v}}{ \thread{\delayedf ~ \eimply{w^*} ~ \constr} }{} \\

\textsf{Delayed formula} & \delayedf &::=& \bigvee ({\bigwedge} \locksetf \wedge \pconstr) \\

%% {\term{p}{::}\predfo{\term{c}}{{\term{v}}^*}{\fracperm}} \\ 

\textsf{Lockset formula} & \locksetf &::=& \nonterm{v} \in \alockset \mid 
\nonterm{v} \notin \alockset \\

\textsf{Pure formula} & \pure &::=& \ldots \mid \mset \\

\textsf{Set formula} & \mset &::=& \mterm_1 \bagsubsume \mterm_2 \mid \mterm_1 = \mterm_2 \hide{\mid \nonterm{v} \in \mterm} \\

\textsf{Set term} & 
	\mterm &::=& \alockset \mid \set{} \mid \set{v} \mid \mterm_1 \bagunion \mterm_2 \mid
	\mterm_1 \bagintersect \mterm_2 \mid \mterm_1 \bagsubtract \mterm_2 \\

\ldots

\end{array}
\]
\savespace
\[
\begin{array}{c}

\term{C} \in \textsf{Data names} \bagunion \{ \code{LOCK} \}

\end{array}
\]

%% \savespace
\savesmallspace
\end{frameit}
%\savespace
\savespace
\caption{Grammar for Core Specification Language with Locks}\label{fig.speclang-locks}
\end{minipage}
%% \savespace\savespace
%% \savespace\savespace
%% \savesmallspace
\end{center}
\end{figure}

%%%%%%%%%%%%%%%%%%%%%%%%%%%%%%%%%%%%%%%%

\input{perm-rules-locks}

Our specification language to support the delayed lockset checking
technique is presented in Fig.~\ref{fig.speclang-locks}.
The preserved variable $\alockset$ is used to keep track
of the lockset of a thread, i.e. $\alockset$ captures
the set of locks held by the thread. The pure formula
$\pure$ additionally contains the set formula
$\mset$ capturing constraints on the content of
the lockset $\alockset$.
Each disjunct of a separation formula $\constr$
now includes a lock formula $\lockf$
indicating the presence and absence of locks
in the lockset $\alockset$.
The key idea of delayed lockset constraints are captured
in the specification of the thread node
\permsto{\term{v}}{ \thread{\delayedf ~ \eimply{w^*} ~ \constr} }{}.
The thread node additionally captures the delayed formula
$\delayedf$ which was delayed at a fork point and will be
checked at a join point.
Sub-structural rules for thread nodes with delayed constraints
are shown in Fig.~\ref{fig.perm-rules-locks}.

\input{fwdrules-locks}

Forward verification rules for supporting the delayed
lockset checking technique are presented in Fig.~\ref{fig.fwdrules-locks}.
When forking a new thread (\entrulen{D-FORK}),
the lockset constraints $\delayedf_{pr}$
in the pre-condition $\constr_{po}$ are not checked
but are filtered out and, together with the post-state $\constr^{'}_{po}$,
they are carried in the newly-created thread node.
The auxiliary function $removeLS$ removes lockset constraints from
the pure formula $\pure$ as they are irrelevant in the context of
the caller. The semantics of $removeLS$ is straightforward,
hence it is not omitted.
The joiner will exchange the thread node for the resource
$\constr^{'}_{po}$ only when the delayed lockset
constraints $\delayedf_{pr}$ are satisfied (\entrulen{D-JOIN-1}).
Joining an already-completed thread is no-op without delayed checking
(\entrulen{D-JOIN-2}).

By capturing the delayed formula in a thread node,
we enable verifying deadlock freedom of the program
shown in Fig.~\ref{fig:outline-locks}.
The program is challenging to verify
as it consists of non-lexical fork/join,
interactions between fork/join/acquire/release,
and multi-join.
We are not aware of any existing verification
systems (including {\sc{ParaHIP}}~\cite{Le:ATVA13}) capable
of verifying this program.
The proof to certify
that the program is deadlock-free is outlined
in Fig.~\ref{fig:outline-locks}.

}

%\newpage
\section{Additional Experimental Results}
\label{sec:experiment-app}

\input{experiment-app}
